# Supplementary material for: Unifying Interacting Nodal Semimetals: A New Route to Strong Coupling
Source: arXiv:1812.05615 ancillary file (2019-11-14)
Supplement: Supplementary file 1 [file ASM_SM_modified.pdf]

# Supplemental Materials: 'Unifying Interacting Nodal Semimetals: A New Route to Strong Coupling'

Shouvik Sur
*Department of Physics & Astronomy, Northwestern University, Evanston, IL 60208, USA*
*National High Magnetic Field Laboratory and Department of Physics, Florida State University, Tallahassee, Florida 32306, USA*

Bitan Roy
*Max-Planck-Institut für Physik komplexer Systeme, Nothnitzer Stra. 38, 01187 Dresden, Germany*
(Dated: April 14, 2019)

We write the $d$-dimensional action from the main text in a more convenient form,

$$S = i \sum_{n=1}^{N_f} \int_k \bar{\psi}_{n,k}\, \sigma_0 \otimes \left[\boldsymbol{k}\cdot\boldsymbol{\gamma} + (|\boldsymbol{K}|^2 + \Delta)\gamma_2\right]\psi_{n,k} + \frac{1}{8}\int_q (|\boldsymbol{Q}|^2 + M^2)\, \mathrm{tr}\left\{\widetilde{\Phi}_{-q}\widetilde{\Phi}_q\right\} + \frac{g\mu^{(3-d)/2}}{\sqrt{N_f}} \sum_{n=1}^{N_f}\int_{k,q} \bar{\psi}_{n,k+q}\widetilde{\Phi}_q\psi_{n,k}. \tag{S1}$$

Here $\boldsymbol{\gamma} = (\gamma_0, \gamma_1) \equiv (\tau_3, \tau_2)$ and $\gamma_2 \equiv -\tau_1$, $\bar{\psi} \equiv \psi^\dagger\gamma_0$, and

$$\widetilde{\Phi} \equiv \begin{cases} \boldsymbol{\phi}(q)\cdot\boldsymbol{\sigma}\otimes\tau_0 & \text{for SDW} \\ \boldsymbol{\phi}(q)\cdot\boldsymbol{\sigma}_\perp\otimes\tau_0 & \text{for SC} \\ \phi(q)\,\sigma_0\otimes\tau_0 & \text{for CDW} \end{cases}. \tag{S2}$$

Thus the fermion propagator used below is $\mathcal{G}_0(k) = -i\sigma_0 \otimes \left[\boldsymbol{k}\cdot\boldsymbol{\gamma} + (|\boldsymbol{K}|^2 + \Delta)\gamma_2\right]^{-1}$. We note that $c$ has been set to 0 as discussed in the main text and below in §I. A brief summary of the content of this supplemental material is as follows:

I. Key features of the formalism 1
II. Resummed boson propagator 2
III. Derivation of the RG equations 3
IV. One-loop Counter-terms 4
V. Importance of damping of the boson's dynamics 6

## I. KEY FEATURES OF THE FORMALISM

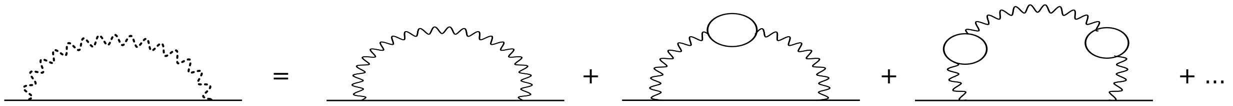

FIG. S1: Implicit resummation of diagrams in the RG analysis that cuts off infrared divergences arising in the $c \to 0$ limit. The dotted (solid) wiggly and solid lines represent the dressed (bare) boson and fermion propagator, respectively.

The tree-level scale invariance of the fermion propagator comes at the cost of $c$ being strongly irrelevant [see Eq. (3) of the main text]. Thus, $c^{-1}$ acts like a momentum scale, regulating divergences in diagrams involving the bare boson propagator. Within a perturbative window the quantum corrections are generally weak, and they cannot compensate a strong negative tree-level scaling dimension, which leads to $c$ flowing to zero. Anticipating this fate, we set $c = 0$ from the outset. This is equivalent to setting the ultraviolet scale of the effective field theory to be lower than the crossover scale below which quantum fluctuations

dominate over the high energy term $c^2|\boldsymbol{q}|^2$. The bosonic propagator then simplifies to $D_0^{-1}(q) = |\boldsymbol{Q}|^2$. In order to obtain a well-defined infrared (IR) scaling limit, physical quantities cannot be singular in $c$ and the spurious divergences arising at $c = 0$ are eliminated once IR adjustments are taken in to account. To this end, we implicitly resum an entire series of diagrams, shown in Fig. S1 [S1]. This procedure is equivalent to replacing each bare boson propagator within a given Feynman diagram by a suitably dressed ultraviolet finite counterpart, and depending on the low energy DoS, it either Landau damps or screens the boson dynamics.

## II. RESUMMED BOSON PROPAGATOR

Here we obtain the expression of the dressed boson propagator $D(q)$ that is valid close to $d = 3$. Since we are after the singular UV finite part of $D(q)$, it is convenient to calculate the polarization bubble at $d = 3$. Setting $\Delta = 0$, at the topological QCP we obtain ($\mu, \nu = 0$: CDW; $\mu, \nu \neq 0$: SDW)

$$\Pi_{\mu\nu}(q) = -g^2 \int \mathrm{d}k\, \mathrm{Tr}\{\mathcal{G}_0(k+q)\sigma_\mu \otimes \tau_0 \mathcal{G}_0(k)\sigma_\nu \otimes \tau_0\}. \tag{S3}$$

Since the trace enforces $\mu = \nu$, $\Pi_{\mu\nu} \propto \delta_{\mu\nu}$. Therefore we directly consider the diagonal part, $\Pi_{\mu\mu}$. We integrate over $\boldsymbol{k}$ by generalizing the dimension of $\boldsymbol{k}$ space to be $2(1-\epsilon_b)$ with $\epsilon_b \to 0^+$. We evaluate Eq. (S3) for general values of $\boldsymbol{q}$ and $\boldsymbol{Q}$ in the presence of a hard UV cutoff $\Lambda$ such that $|\boldsymbol{K}| \leq \Lambda$. It is convenient to scale out $\boldsymbol{q}$ such that $|\boldsymbol{K}| \mapsto \sqrt{z|\boldsymbol{q}|}$, and define the scaled momentum $\widetilde{Q} = |\boldsymbol{Q}|/\sqrt{|\boldsymbol{q}|}$ and UV cutoff $\widetilde{\Lambda} = \Lambda/\sqrt{|\boldsymbol{q}|}$. Integrating over $\boldsymbol{K}$ leads to

$$\Pi_{\mu\mu}(\boldsymbol{q},\boldsymbol{Q}) = \frac{g^2|\boldsymbol{q}|}{(2\pi)^2}\Big[\widetilde{\Lambda}^2(\epsilon_b^{-1} - \ln|\boldsymbol{q}|^2) - \widetilde{\Lambda}^2\left(\log\left(\widetilde{\Lambda}^4+1\right)-2\right) - 2\tan^{-1}\left(\widetilde{\Lambda}^2\right) - \widetilde{Q}^2\sinh^{-1}(\widetilde{\Lambda}^2) + F(\widetilde{Q},\widetilde{\Lambda})\Big], \tag{S4}$$

where $F(\widetilde{Q},\widetilde{\Lambda}) = \int_{-\pi}^{\pi}\frac{\mathrm{d}\theta}{2\pi}\int_0^{\widetilde{\Lambda}^2}\mathrm{d}z\, f(z,\theta,\widetilde{Q})$, with $f(z,\theta,\widetilde{Q})$ being a real-valued function that asymptotically behaves as

$$f(z,\theta,\widetilde{Q}) = \begin{cases} \mathcal{O}\left(z^0\right), & \text{for } z \ll 1 \\ \dfrac{\widetilde{Q}^2(\cos(\theta)-\cos(2\theta))}{6z} + \mathcal{O}\left(z^{-2}\right), & \text{for } z \gg 1 \end{cases}. \tag{S5}$$

Since in the $z \to \infty$ limit the coefficient of the $\mathcal{O}(1/z)$ term vanishes upon angular integration, $\int \mathrm{d}\theta\, \mathrm{d}z\, f(z,\theta,\widetilde{Q})$ is UV finite, and expected to be IR finite (we demonstrate these explicitly below).

Since $F(\widetilde{Q},\widetilde{\Lambda})$ is UV finite and we are interested in the $\mathcal{O}\left(\widetilde{\Lambda}^0\right)$ contribution of $F(\widetilde{Q},\widetilde{\Lambda})$, let us define, $F_\infty(\widetilde{Q}) = \lim_{\widetilde{\Lambda}\to\infty} F(\widetilde{Q},\widetilde{\Lambda})$. It is difficult to analytically calculate $F_\infty(\widetilde{Q})$. So we propose the ansatz

$$F_\infty(\widetilde{Q}) = \left(\pi - \frac{\pi^2}{4}\right) + \widetilde{Q}^2\left[\log\left(\widetilde{Q}^2 + \frac{5\pi}{6}\right) - \frac{4}{5}\right]. \tag{S6}$$

In Fig. S2 we compare the numerically evaluated values of $F_\infty(\widetilde{Q})$ with the ansatz over the range $\widetilde{Q} \in (10^{-4}, 3\times 10^2)$. Due to the excellent match over several decades of $\widetilde{Q}$, we conclude

$$\begin{aligned}\Pi_{\mu\mu}(\boldsymbol{q},\boldsymbol{Q}) = {}& \frac{g^2\Lambda^2}{(2\pi)^2}(\epsilon_b^{-1} + 2 - 2\ln\Lambda^2) \\ &+ \frac{g^2}{(2\pi)^2}\left[-\frac{\pi^2}{4}|\boldsymbol{q}| + |\boldsymbol{Q}|^2\ln\left(\frac{|\boldsymbol{Q}|^2}{|\boldsymbol{q}|} + \frac{5\pi}{6}\right) - |\boldsymbol{Q}|^2\ln\frac{\Lambda^2}{|\boldsymbol{q}|} - \left(\frac{4}{5}+\ln 2\right)|\boldsymbol{Q}|^2 + \mathcal{O}\left(\frac{|\boldsymbol{q}|}{\Lambda^2}\right)\right].\end{aligned} \tag{S7}$$

It is important to note that the regulator $\epsilon_b$ only affects the quantum correction to the boson's mass. Moreover, the coefficients of the $\ln\Lambda$ terms are independent of $\epsilon_b$, which implies that the regularization of the UV divergence in $\boldsymbol{k}$-space does not affect the RG flow at one-loop order close to $d = 3$. It can be verified that the three limiting cases obtained from Eq. (S7)

$$\lim_{q\to 0}\lim_{Q\to 0}\Pi_{\mu\mu}(\boldsymbol{q},\boldsymbol{Q}) = \frac{g^2\Lambda^2}{(2\pi)^2}(\epsilon_b^{-1} + 2 - 2\ln\Lambda^2); \quad \lim_{Q\to 0}\Pi_{\mu\mu}(\boldsymbol{q},\boldsymbol{Q}) = -\frac{g^2|\boldsymbol{q}|}{16}; \tag{S8}$$

$$\lim_{q\to 0}\Pi_{\mu\mu}(\boldsymbol{q},\boldsymbol{Q}) = -\frac{g^2|\boldsymbol{Q}|^2}{(2\pi)^2}\left[\ln\frac{\Lambda^2}{|\boldsymbol{Q}|^2} + \mathcal{O}(1)\right], \tag{S9}$$

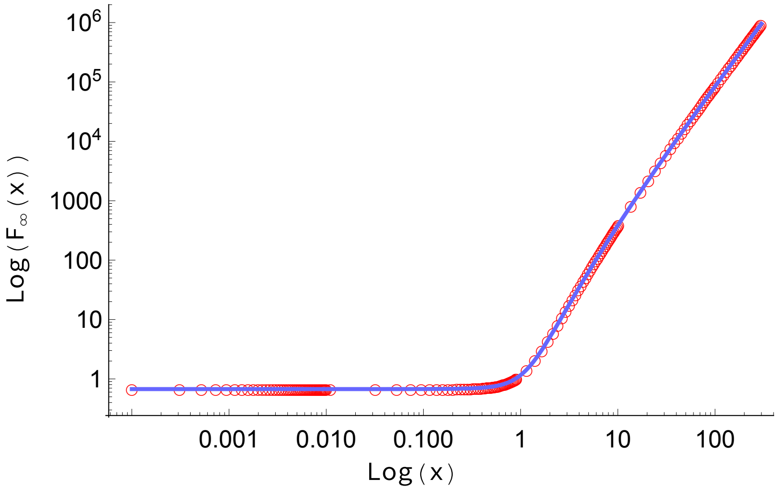


FIG. S2: Comparison between numerically evaluated values of $F_\infty(x)$ and the ansatz in Eq. (S6). The solid (blue) line is the plot of the ansatz, while the empty circles are numerically evaluated values of $F_\infty(x)$.

match the results obtained from explicitly calculating $\Pi_{\mu\mu}(\boldsymbol{q},\boldsymbol{Q})$ at (i) $q=0$; (ii) $\boldsymbol{Q}=\boldsymbol{0}$; (iii) $\boldsymbol{q}=\boldsymbol{0}$, which lends further support to our ansatz.

## III. DERIVATION OF THE RG EQUATIONS

Since all 4 terms in Eq. (S1) are perturbatively renormalizable, we add the corresponding counterterms (defined as *negative* of the quantum corrections) to obtain the renormalized action

$$S_{ren} = i\int \mathrm{d}k\,\psi^\dagger(k)\sigma_0\otimes\left[\mathcal{Z}_1\boldsymbol{k}\cdot\boldsymbol{\gamma}+\mathcal{Z}_2|\boldsymbol{K}|^2\gamma_2\right]\psi(k)+\frac{1}{8}\int \mathrm{d}q\,\mathcal{Z}_3|\boldsymbol{Q}|^2\,\mathrm{tr}\{\Phi(-q)\Phi(q)\}$$
$$+\mu^{\frac{3-d}{2}}g\mathcal{Z}_4\int \mathrm{d}k\,\mathrm{d}q\,\psi^\dagger(k+q)\widetilde{\Phi}(q)\psi(k), \tag{S10}$$

where $\mathcal{Z}_n = 1+\sum_{m=1} Z_{nm}\epsilon^{-m}$. By expressing $S_{ren}$ in terms of bare quantities we obtain their relationship with the renormalized counterparts

$$\boldsymbol{k}_B = \mathcal{Z}_{\boldsymbol{k}}^{-1}\boldsymbol{k},\qquad \boldsymbol{K}_B=\boldsymbol{K}_B,\qquad \psi_B=\sqrt{\mathcal{Z}_\psi}\,\psi,\qquad \phi_B=\sqrt{\mathcal{Z}_\phi}\,\phi,\qquad g_B=\mu^{\frac{3-d}{2}}\frac{\mathcal{Z}_{\boldsymbol{k}}^4\mathcal{Z}_4}{\mathcal{Z}_\psi\sqrt{\mathcal{Z}_\phi}}\,g, \tag{S11}$$

where $\mathcal{Z}_{\boldsymbol{k}}=\mathcal{Z}_2/\mathcal{Z}_1$, $\mathcal{Z}_\psi=\mathcal{Z}_2\mathcal{Z}_{\boldsymbol{k}}^2$, and $\mathcal{Z}_\phi=\mathcal{Z}_3\mathcal{Z}_{\boldsymbol{k}}^2$. The anisotropy exponent ($z_{\boldsymbol{k}}$) and the anomalous dimensions of the fields are defined as

$$z_{\boldsymbol{k}} = 2-\frac{\partial\ln\mathcal{Z}_{\boldsymbol{k}}}{\partial\ln\mu},\qquad \eta_\psi=\frac{1}{2}\frac{\partial\ln\mathcal{Z}_\psi}{\partial\ln\mu},\qquad \eta_\phi=\frac{1}{2}\frac{\partial\ln\mathcal{Z}_\phi}{\partial\ln\mu}, \tag{S12}$$

while the beta-function of $g$ for its flow along increasing $\mu$ is obtained from, $\frac{\partial g_B}{\partial\ln\mu}=0$. This leads to a set of coupled equations,

$$\begin{aligned}&\mathcal{Z}_1\mathcal{Z}_2(z_{\boldsymbol{k}}-2)+(\mathcal{Z}_1\partial_g\mathcal{Z}_2-\mathcal{Z}_2\partial_g\mathcal{Z}_1)\beta_g=0,\qquad 2\mathcal{Z}_2[\eta_\psi+(z_{\boldsymbol{k}}-2)]-\beta_g\partial_g Z_2=0,\\ &2\mathcal{Z}_3[\eta_\phi+(z_{\boldsymbol{k}}-2)]-\beta_g\partial_g Z_3=0,\qquad (g\partial_g\mathcal{Z}_4+\mathcal{Z}_4)\beta_g+g\mathcal{Z}_4[(3-d)/2-4(z_{\boldsymbol{k}}-2)-2\eta_\psi-\eta_\phi]=0,\end{aligned} \tag{S13}$$

where $\beta_g\equiv\mu\frac{\partial g}{\partial\mu}$. We set $d=3-\epsilon$ and solve these equations to obtain,

$$\begin{aligned}&z_{\boldsymbol{k}}=2-\frac{1}{2}g\partial_g(Z_{11}-Z_{21}),\qquad \eta_\psi=-\frac{1}{4}g\partial_g Z_{21}-(z_{\boldsymbol{k}}-2),\qquad \eta_\phi=-\frac{1}{4}g\partial_g Z_{31}-(z_{\boldsymbol{k}}-2),\\ &\beta_g=g\left[-\frac{\epsilon}{2}+4(z_{\boldsymbol{k}}-2)+2\eta_\psi+\eta_\phi\right]+\frac{1}{2}g^2\partial_g\mathcal{Z}_{41}.\end{aligned} \tag{S14}$$

We deduce that while the vertex correction produces a quantum correction, the various self-energies generate an anomalous dimension of the Yukawa vertex. The flow towards IR, i.e. decreasing energy is obtained from the relation, $\partial_\ell g = -\beta_g$.

## IV. ONE-LOOP COUNTER-TERMS

### A. Fermion self-energy: $Z_{11}$ and $Z_{21}$

$Z_{11}$ and $Z_{21}$ are obtained from the one-loop fermion self-energy. We use the dressed boson propagator, $D^{-1}(q) = Ag^2|\boldsymbol{q}| + |\boldsymbol{Q}|^2$, where $A = 1/16$, and write the bare fermion propagator as $\mathcal{G}_0(k) = \sigma_0 \otimes \mathfrak{G}_0(k)$ with $\mathfrak{G}_0(k) = -i\,\frac{\boldsymbol{k}\cdot\boldsymbol{\gamma}+|\boldsymbol{K}|^2\gamma_2}{|\boldsymbol{k}|^2+|\boldsymbol{K}|^4}$. Thus the fermion self-energy is given by

$$\Sigma(k) = \frac{N_b g^2}{N_f}\sigma_0 \otimes \int \mathrm{d}q\, \mathfrak{G}_0(k+q) D(q) = -i\frac{N_b g^2}{N_f}\sigma_0 \otimes \int \mathrm{d}q\, \frac{(\boldsymbol{k}+\boldsymbol{q})\cdot\boldsymbol{\gamma} + |\boldsymbol{K}+\boldsymbol{Q}|^2\gamma_2}{|\boldsymbol{k}+\boldsymbol{q}|^2 + |\boldsymbol{K}+\boldsymbol{Q}|^4} \frac{1}{Ag^2|\boldsymbol{q}| + |\boldsymbol{Q}|^2}. \tag{S15}$$

At the topological QCP, $\Sigma(0)$ vanishes due to the Veltman formula in $d_Q = 2-\epsilon$ dimensions. Therefore, assuming proximity to the upper critical dimension, we evaluate $\Sigma(k)$ in the two limiting cases, (1) $\boldsymbol{K} = \boldsymbol{0}$; (2) $\boldsymbol{k} = \boldsymbol{0}$.

#### *1.* $\mathbf{K} = \mathbf{0}$

Here we have to deal with three vectors: $\boldsymbol{q}$, $\boldsymbol{k}$, and $\boldsymbol{\gamma}$, which leads to 2 independent angles. Let us define $\hat{k}\cdot\hat{q} = \cos\theta_q$, and scale $|\boldsymbol{q}| \mapsto y|\boldsymbol{Q}|^2$. The self-energy takes the form

$$\Sigma(\boldsymbol{k}) = -i\frac{N_b g^2}{N_f}\sigma_0 \otimes \int \mathrm{d}\boldsymbol{Q} \int_0^\infty \frac{dy}{2\pi}\frac{y}{(Ag^2)y+1}\int_0^{2\pi}\frac{d\theta_q}{2\pi}\frac{(y\cos\theta_q + \frac{|\boldsymbol{k}|}{|\boldsymbol{Q}|^2})\hat{k}\cdot\boldsymbol{\gamma} + \gamma_2}{y^2 + \left(\frac{|\boldsymbol{k}|}{|\boldsymbol{Q}|^2}\right)^2 + 1 + 2y\frac{|\boldsymbol{k}|}{|\boldsymbol{Q}|^2}\cos\theta_q}. \tag{S16}$$

After integrating over $\theta_q$ we isolate those terms that diverge in the $\epsilon \to 0$ limit to obtain

$$\Sigma(\boldsymbol{k}) = -i\frac{N_b g^2}{N_f}\sigma_0 \otimes \int \mathrm{d}\boldsymbol{Q}\int_0^\infty \frac{dy}{2\pi}\frac{y}{(Ag^2)y+1}\left[\frac{\gamma_2}{y^2+1} + \frac{1}{(y^2+1)^2}\frac{\boldsymbol{k}\cdot\boldsymbol{\gamma}}{|\boldsymbol{Q}|^2+|\boldsymbol{k}|}\right] + \ldots, \tag{S17}$$

where '…' refers to terms that are finite in the $\epsilon \to 0$ limit. The first term vanishes due to the Veltman formula. In the limit $(Ag^2) \ll 1$, the second term leads to

$$\Sigma(\boldsymbol{k}) = -i\frac{2N_b g^2}{(4\pi)^2 N_f \epsilon}\sigma_0 \otimes \boldsymbol{\gamma}\cdot\boldsymbol{k}, \tag{S18}$$

which implies,

$$Z_{11} = -\frac{N_b g^2}{2(2\pi)^2 N_f}. \tag{S19}$$

Thus the damping does not affect $Z_{11}$ at leading order in $g^2$.

#### *2.* $\mathbf{k} = \mathbf{0}$

First we integrate over $\boldsymbol{q}$ by scaling, $|\boldsymbol{q}| \mapsto \frac{|\boldsymbol{Q}|^2}{Ag^2}y$. The self-energy takes the form

$$\Sigma(\boldsymbol{K}) = -i\frac{N_b g^2}{N_f}\sigma_0 \otimes \int \frac{\mathrm{d}\boldsymbol{Q}}{|\boldsymbol{Q}|^2}\int_0^\infty \frac{dy}{2\pi}\frac{y}{y+1}\frac{|\boldsymbol{K}+\boldsymbol{Q}|^2\gamma_2}{y^2 + \left(\frac{Ag^2|\boldsymbol{K}+\boldsymbol{Q}|^2}{|\boldsymbol{Q}|^2}\right)^2} \tag{S20}$$

$$= -i\frac{N_b g^2}{4\pi N_f}\sigma_0 \otimes \int \mathrm{d}\boldsymbol{Q}\,\frac{|\boldsymbol{K}+\boldsymbol{Q}|^2}{|\boldsymbol{Q}|^4 + (Ag^2)^2|\boldsymbol{K}+\boldsymbol{Q}|^4}\left(2|\boldsymbol{Q}|^2\ln\frac{|\boldsymbol{Q}|^2}{Ag^2|\boldsymbol{Q}+\boldsymbol{K}|^2} + \pi(Ag^2)|\boldsymbol{Q}+\boldsymbol{K}|^2\right). \tag{S21}$$

Using the relation $\ln\left(1+a^{-1}\right) = \int_0^1 \mathrm{d}x\,(x+a)^{-1}$ we integrate over $\boldsymbol{Q}$, and in the limit $Ag^2 \ll 1$ we obtain

$$\Sigma(\boldsymbol{K}) = -i\frac{N_b g^2}{N_f}\frac{\sigma_0 \otimes \gamma_2}{(2\pi)^2\epsilon}\left(\ln\frac{1}{Ag^2} - 2\right)|\boldsymbol{K}|^2. \tag{S22}$$

Therefore,

$$Z_{21} = -\frac{N_b g^2}{(2\pi)^2 N_f}\left(\ln\frac{1}{Ag^2} - 2\right). \tag{S23}$$

### B. Boson self-energy: $Z_{31}$

This calculation is identical to the one in Appendix II up to the integration over $\boldsymbol{k}$. Since we are after the coefficient of the $|\boldsymbol{Q}|^2$ in the boson propagator we set $\boldsymbol{q}=0$ to obtain

$$\Pi_{\mu,\mu}(\boldsymbol{Q}) = -\frac{g^2}{\pi}\int \mathrm{d}\boldsymbol{K}\left[\frac{\boldsymbol{Q}\cdot\boldsymbol{K}}{|\boldsymbol{K}|^2+|\boldsymbol{Q}|^2/4}\ln\left(\frac{|\boldsymbol{K}+\boldsymbol{Q}|^2}{|\boldsymbol{K}-\boldsymbol{Q}|^2}\right) + \ln\left((|\boldsymbol{K}|^2+|\boldsymbol{Q}|^2/4)^2 - (\boldsymbol{K}\cdot\boldsymbol{Q})^2\right) - \epsilon_b^{-1}\right]. \tag{S24}$$

We subtract the boson mass renormalization, $\Pi_{\mu,\mu}(0)$, and find that only the first term carries a $\epsilon^{-1}$ dependence. We evaluate to obtain

$$\Pi_{\mu,\mu}(\boldsymbol{Q}) - \Pi_{\mu,\mu}(0) = -\frac{2g^2}{(2\pi)^2\epsilon}|\boldsymbol{Q}|^2, \tag{S25}$$

which leads to

$$Z_{31} = -\frac{2g^2}{(2\pi)^2}. \tag{S26}$$

### C. Vertex correction: $Z_{41}$

In this appendix we present the calculation for one-loop vertex correction. For $N_b=2$ the vertex correction vanishes because $\sum_{i=1,2}\sigma_i\sigma_j\sigma_i = 0$, so we here focus on $N_b = 1$ and 3. The quantum correction takes the form

$$\delta S_I\Big|_{CDW} = -(-g/\sqrt{N_f})^3\int \mathrm{d}q\,\mathrm{d}k\,\phi(q)\psi^\dagger(k+q)\Gamma_{CDW}(k,q)\psi(k), \tag{S27}$$

$$\delta S_I\Big|_{SDW} = -(-g/\sqrt{N_f})^3\int \mathrm{d}q\,\mathrm{d}k\,\vec{\phi}(q)\cdot\psi^\dagger(k+q)\vec{\Gamma}_{SDW}(k,q)\psi(k), \tag{S28}$$

for the CDW and SDW criticalities, respectively. Here

$$\Gamma_{CDW}(k,q) = \sigma_0\otimes W(k,q), \qquad \vec{\Gamma}_{SDW}(k,q) = -\vec{\sigma}\otimes W(k,q), \tag{S29}$$

where

$$W(k,q) = \int \mathrm{d}p\,\mathfrak{G}_0(p+q)\mathfrak{G}_0(p)D(k-p). \tag{S30}$$

Since we are interested only in the UV divergent piece, we calculate

$$W(0,\boldsymbol{Q}) = (-i)^2\int \mathrm{d}p\,\frac{\boldsymbol{p}\cdot\boldsymbol{\gamma} + |\boldsymbol{P}+\boldsymbol{Q}|^2\gamma_2}{|\boldsymbol{p}|^2+|\boldsymbol{P}+\boldsymbol{Q}|^4}\,\frac{\boldsymbol{p}\cdot\boldsymbol{\gamma}+|\boldsymbol{P}|^2\gamma_2}{|\boldsymbol{p}|^2+|\boldsymbol{P}|^4}\,\frac{1}{Ag^2|\boldsymbol{p}|+|\boldsymbol{P}|^2} \tag{S31}$$

$W(0,\boldsymbol{Q})$ is evaluated in analogy to the self-energy corrections, and in the $Ag^2 \ll 1$ limit we obtain

$$W(0,\boldsymbol{Q}) = \frac{\tau_0}{2\pi}\ln\left(Ag^2\right)\int \mathrm{d}\boldsymbol{P}\,\frac{|\boldsymbol{P}|^2}{|\boldsymbol{P}|^4+(Ag^2)^2|\boldsymbol{Q}+\boldsymbol{P}|^4} + \mathcal{O}\left(g^2\right). \tag{S32}$$

Since by power-counting the integral is at most logarithmically divergent in $d = 3$, the precise form of the second term in the denominator plays a sub-dominant role in the determination of the coefficient of the $1/\epsilon$ term in the small $g^2$ limit . Thus we approximate it by $|\boldsymbol{Q} + \boldsymbol{P}|^4 \mapsto |\boldsymbol{Q} + \boldsymbol{P}|^2 |\boldsymbol{P}|^2$, to obtain

$$W(0, \boldsymbol{Q}) = \frac{\tau_0}{(2\pi)^2 \epsilon} \big[\ln\big(Ag^2\big) + \mathcal{O}\left(Ag^2\right)\big]. \tag{S33}$$

Therefore,

$$Z_{41} = \frac{(N_b - 2)}{N_f} \frac{g^2}{(2\pi)^2} \big[\ln\big(Ag^2\big) + \mathcal{O}\left(Ag^2\right)\big]. \tag{S34}$$

## V. IMPORTANCE OF DAMPING OF THE BOSON'S DYNAMICS

Here we demonstrate that the dynamically generated damping term plays an essential role in the determination of the asymptotic scaling behavior. We also show that a naive perturbative expansion around the non-interacting fixed point either leads to large quantum corrections in the *correct* low energy limit which invalidates the use of perturbation theory, or in an incorrect low energy limit $(\ln \Lambda)^2$ terms are generated which cannot be resummed and an RG treatment of the problem becomes invalid.

We use the quantum correction to $\Delta$, resulting from $\Sigma(0)$, to demonstrate the aforementioned features. Since $\Sigma(0)$ vanishes by the Veltman formula in $d = 3 - \epsilon$ at the topological QCP, we compute it in $d = 3$ to explicitly obtain the quantum correction to $\Delta$, and show that it is finite and does not carry any $\ln(\Lambda)$ dependence when the damping is taken into account.

After the angular integrations in the $\boldsymbol{q}$ and $\boldsymbol{Q}$ planes we obtain

$$\Sigma(0) = -i \frac{g^2}{(2\pi)^2} \sigma_0 \otimes \gamma_2 \int_0^\Lambda \mathrm{d}Q_r\, Q_r \int_0^\infty \mathrm{d}q_r\, q_r \frac{Q_r^2}{(q_r^2 + Q_r^4)(Ag^2 q_r + Q_r^2)}, \tag{S35}$$

where $Q_r$ ($q_r$) is the radial component of $\boldsymbol{Q}$ ($\boldsymbol{q}$). We integrate over $q_r$ first followed by $Q_r$ to obtain

$$\Sigma(0) = -i\, \frac{g^2 \Lambda^2}{(4\pi)^2}\, \frac{\pi A g^2 - 2\ln\big(Ag^2\big)}{2(1 + (Ag^2)^2)}\, \sigma_0 \otimes \gamma_2. \tag{S36}$$

Thus in the weak-coupling limit ($Ag^2 \ll 1$)

$$\Sigma(0) \approx i\, \frac{2g^2 \Lambda^2 \ln\big(Ag^2\big)}{(4\pi)^2}\, \sigma_0 \otimes \gamma_2. \tag{S37}$$

Regarding Eq. (S37) we note:

1. $\Sigma(0)$ is logarithmically enhanced due to the damping term in the boson propagator.

2. There is no $\ln \Lambda$ dependence, and apparently it has been replaced by $\ln\left(Ag^2\right)$. This is a non-trivial feature of the low-energy limit that we take. To further illustrate this key aspect let us calculate the 1-loop self-energy generated by the bare boson propagator, $D_0^{-1}(q) = c^2 q_r^2 + Q_r^2$, in which case (changing $Q_r \mapsto x/c$)

$$\Sigma_0(0) = g^2 \sigma_0 \otimes \int \mathrm{d}q\, \mathfrak{G}_0(k+q) D_0(q) = -i \frac{g^2}{(2\pi)^2} \sigma_0 \otimes \gamma_2 \int_0^{c\Lambda} \mathrm{d}x\, \frac{x \ln x}{x^2 - 1}. \tag{S38}$$

Note that $c\Lambda \equiv \widetilde{c}$ is a dimensionless parameter, whose magnitude determines 3 distinct cases,

$$\widetilde{c} \ll 1\text{: } \Sigma(0) = i\, \frac{2g^2\Lambda^2}{(4\pi)^2} \left[\ln \widetilde{c} + \mathcal{O}\left(\widetilde{c}^0\right)\right] \sigma_0 \otimes \gamma_2, \tag{S39}$$

$$\widetilde{c} = 1\text{: } \Sigma(0) = -i\, \frac{\pi^2 g^2 \Lambda^2}{6(4\pi)^2}\, \sigma_0 \otimes \gamma_2, \tag{S40}$$

$$\widetilde{c} \gg 1\text{: } \Sigma(0) = -i\, \frac{g^2}{(4\pi)^2 c^2} \left[(\ln \widetilde{c})^2 + \mathcal{O}\left(1\right)\right] \sigma_0 \otimes \gamma_2. \tag{S41}$$

Since $c$ is an irrelevant parameter, $\partial_\ell \widetilde{c} = -\widetilde{c}$ at tree-level, which implies that within a perturbative RG, generally, it cannot obtain a stable fixed point. Therefore, the appropriate low energy limit corresponds to $\widetilde{c} = c\Lambda \to 0$. The behavior in

Eq. (S37) is consistent with the case $\widetilde{c} \ll 1$ as long as $\widetilde{c}$ is finite, because the divergence in the $\widetilde{c} \to 0$ limit is cut off by the quantum correction generated by the polarization bubble which leads to the singular $\ln\left(Ag^2\right)$ dependence of $\Sigma(0)$. Therefore, taking $\Lambda \to \infty$ at fixed $c$ leads to an incorrect low-energy limit: $\widetilde{c} \gg 1$, where the non-resummable $(\ln \Lambda)^2$ term arises. In fact, the appearance of similar log-squared term in the fermion self-energy leads to differences in the approaches and results of Refs. [S2] and [S3], where the authors studied the scaling behavior of ASMs in the presence of only long-range Coulomb interaction. Although we studied a completely different critical system, Landau damping still plays a key role at low energies due to the anisotropic scaling dictated by the fermionic dynamics. Here we agree with the diagnosis offered by Ref. [S3], and conclude that the correct low energy limit will not lead to log-squared terms.

[S1] D. Dalidovich and S.-S. Lee, Phys. Rev. B **88**, 245106 (2013).
[S2] G. Y. Cho and E.-G. Moon, Sci. Rep. **6**, 19198 (2016).
[S3] H. Isobe, B.-J. Yang, A. Chubukov, J. Schmalian, and N. Nagaosa, Phys. Rev. Lett. **116**, 076803 (2016).
